# Supplementary material for: Robotouille: An Asynchronous Planning Benchmark for LLM Agents
Source: arXiv:2502.05227 source file (2025-02-06)
Supplement: Supplementary file 1 [file gemini_discussion.tex]

\NS{In this section, we qualitatively highlight that the Gemini model performs poorly with \react{} because it erroneously plans to solve the goal of the few-shot example rather than the current environment goal. We suspect this is due to the long context length of the \react{} few-shot example compared to the examples for \io{} and \iocot{}. This aligns with findings in \cite{liu2023lostmiddlelanguagemodels} where LLMs have been observed to perform poorly in long-context tasks.}
