# Supplementary material for: Robotouille: An Asynchronous Planning Benchmark for LLM Agents
Source: arXiv:2502.05227 source file (2025-02-06)
Supplement: Supplementary file 2 [file open_source_results.tex]

\NS{In this section, we have included new experiments on task 1 of the synchronous setting using top-performing open-source LLMs on the HuggingFace LLM leaderboard. The following experiments were run on 4 NVIDIA RTX 6000 Adas using FP8 quantization.}

\begin{table}[h]
    \small
    \centering
    \begin{tabular}{lc}
        \toprule
        & \textbf{Synchronous (\%) $\pm$ SE} \\ 
        \midrule
        \texttt{gemma-2-27b-it} & 20.0 $\pm$ 12.0 \\
        \texttt{gemma-2-9b-it} & 0.00 $\pm$ 0.00 \\
        \texttt{Meta-Llama-3.1-70b-Instruct} & 30.0 $\pm$ 13.8 \\
        \texttt{Meta-Llama-3.1-8b-Instruct} & 10.0 $\pm$ 9.10 \\
        \texttt{Qwen2-72B-Instruct} & 60.0 $\pm$ 14.8 \\
        \texttt{Qwen2-32B-Instruct} & 50.0 $\pm$ 15.1 \\
        \bottomrule
    \end{tabular}
    \caption{Success rates of state-of-the-art open-source LLMs on the synchronous and asynchronous datasets.}
    \label{tab:open-source}
\end{table}
