# Supplementary material for: Robotouille: An Asynchronous Planning Benchmark for LLM Agents
Source: arXiv:2502.05227 source file (2025-02-06)
Supplement: Supplementary file 3 [file prompts_details.tex]

We use the following instructions for the \io{}, \iocot{}, and \react{} baselines in both the synchronous and asynchronous datasets. Each method is few-shot prompted with an example optimal trajectory on a task unique to the dataset being evaluated on. Notably, the asynchronous example involves a time delay. We ensured that prompt formatting in both datasets was consistent. \react{} example observations are omitted to make experiments cheaper and because we did not note a major difference in performance during preliminary testing.

% Prompt stuff below

\newcolumntype{P}[1]{>{\centering\arraybackslash}p{#1}}
\definecolor{backcolour}{rgb}{	.98, .925, .824}

\tcbset{
listing engine=minted,
    % minted style=trac,
    listing only,
    boxrule=0.1pt,
  minted options={
    fontsize=\scriptsize, % Change font size, use \tiny, \scriptsize, \footnotesize, \small, \normalsize, \large, \Large, \LARGE, \huge, or \Huge
    breaklines=True,
  },
}
\lstset{%
    basicstyle=\small\ttfamily\bfseries,
    % frame=single, % adds a frame around the code
    % backgroundcolor=\color[gray]{0.9}, % sets the background color to light grey
    breaklines=true, % enables line breaking
    postbreak=\mbox{\textcolor{black}{$\hookrightarrow$}\space} % indicator for line breaks
}
\newcommand{\mytcbinput}[4]{
\tcbinputlisting{
      listing file=#1,
      minted options={
        highlightlines={#3}, % Highlight specified lines
        highlightcolor=yellow,
        breaklines=True,        
        fontsize=\scriptsize,
        escapeinside=||,
      },
      breakable,
      title=#2,
      label=lst:#4
    }
}

\mytcbinput{prompts/io_prompt.tex}{I/O Prompt}{0}{io}

\mytcbinput{prompts/io_example_sync.tex}{I/O Synchronous Example}{0}{iosync}

\mytcbinput{prompts/io_example_async.tex}{I/O Asynchronous Example}{0}{ioasync}

\mytcbinput{prompts/iocot_prompt.tex}{I/O CoT Prompt}{0}{iocot}

\mytcbinput{prompts/iocot_example_sync.tex}{I/O CoT Synchronous Example}{0}{iocotsync}

\mytcbinput{prompts/iocot_example_async.tex}{I/O CoT Asynchronous Example}{0}{iocotasync}

\mytcbinput{prompts/react_prompt.tex}{ReAct Prompt}{0}{react}

\mytcbinput{prompts/react_prior_prompt}{ReAct + Prior (appended to ReAct}{0}{react_prior}

\mytcbinput{prompts/react_example_sync.tex}{ReAct Synchronous Example}{0}{react_sync}

\mytcbinput{prompts/react_example_async.tex}{ReAct Asynchronous Example}{0}{react_async}
