# Supplementary material for: Robotouille: An Asynchronous Planning Benchmark for LLM Agents
Source: arXiv:2502.05227 source file (2025-02-06)
Supplement: Supplementary file 4 [file na_qualititative_example.tex]

In this environment, the agent is tasked to make a cheese chicken sandwich, where the chicken needs to be cooked. In order to be most efficient, the agent should prioritise the chicken, first leaving the chicken to cook before stacking the cheese onto the bottom bread. This means that the agent will use less steps to complete the environment because it can begin assembling the sandwich while it is waiting for the chicken to cook. However, in the environment, due to procedural generation, the cheese is initially on top of the stove. Thus, asynchronous planning is not optimal because the agent needs to clear the stove before it can cook the chicken. The most optimal plan would be to stack the cheese immediately when it clears the stove. (Figure 7)

\begin{figure}[t!]
    \centering
    \includegraphics[width=\textwidth]{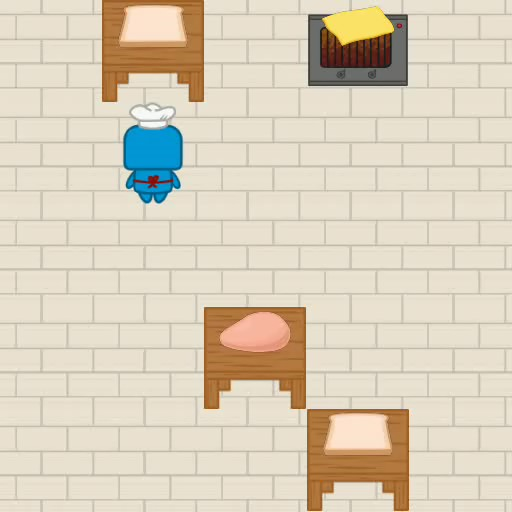}
    \caption{0\_ cheese\_ chicken\_ sandwich\_ 336: Asynchronous planning not possible}
    \label{fig:piechart_followup}
\end{figure}
