# Supplementary material for: Robotouille: An Asynchronous Planning Benchmark for LLM Agents
Source: arXiv:2502.05227 source file (2025-02-06)
Supplement: Supplementary file 5 [file additional_jsons.tex]

\begin{figure}[ht]
    \centering
    % Left column (longest JSON)
    \noindent
    \begin{minipage}[t]{0.48\textwidth}  % Left column (long JSON)
        \vspace{0pt}  % Align at the top of the column
        \begin{tcolorbox}[colframe=black, boxrule=0.5mm, width=\textwidth, boxsep=0pt, left=0pt, right=0pt, top=0pt, bottom=0pt]
        \begin{minted}[fontsize=\scriptsize, breaklines, frame=none, bgcolor=white,
            xleftmargin=0pt, xrightmargin=0pt, texcomments=true, escapeinside=||,
            highlightlines=true, style=colorful, 
            highlightcolor=\color{red}, highlightcolor=\color{green}] {json}
{
    "version": "1.0.0",

    "player": {
        "robot": {
            "front": "robot_front.png",
            "back": "robot_back.png",
            "left": "robot_left.png",
            "right": "robot_right.png"
        }
    },

    "floor": "floorkitchen.png",

    "item": {
        "constants": {
            "STATION_ITEM_OFFSET" : 0.25,
            "X_SCALE_FACTOR": 0.125,
            "Y_SCALE_FACTOR": 0.75
        },
        "entities": {
            "chicken": {
                "assets": {
                    "default": "chicken.png",
                    "cooked": {
                        "asset": "cookedchicken.png",
                        "predicates": ["iscooked"]
                    },
                    "fried": {
                        "asset": "friedchicken.png",
                        "predicates": ["isfried"]
                    }
                },
                "constants": {}
            }, ...
        }
    },

    "station": {
        "constants": {},
        "entities": {
            "fryer": {
                "assets": {
                    "default": "fryer.png"
                },
                "constants": {}
            },...
        }
    },
}
        \end{minted}
        \end{tcolorbox}
    \end{minipage}
    \hfill
    % Right column (stacked two JSONs)
    \begin{minipage}[t]{0.48\textwidth}  % Right column
        \vspace{0pt}
        % First stacked JSON
        \begin{tcolorbox}[colframe=black, boxrule=0.5mm, width=\textwidth, boxsep=0pt, left=0pt, right=0pt, top=0pt, bottom=0pt]
        \begin{minted}[fontsize=\scriptsize, breaklines, frame=none, bgcolor=white,
            xleftmargin=0pt, xrightmargin=0pt, texcomments=true, escapeinside=||,
            highlightlines=true, style=colorful, 
            highlightcolor=\color{red}, highlightcolor=\color{green}] {json}
{
    "version": "1.0.0",
    "width": 3,
    "height": 3,
    "config": {
        "num_cuts": {
            "lettuce": 3,
            "default": 3
        },
        "cook_time": {
            "patty": 3,
            "default": 3
        }
    },
    "stations": [
        {
            "name": "board",
            "x": 0,
            "y": 1,
            "id": "A"
        }
    ],
    "items": [
        {
            "name": "lettuce",
            "x": 0,
            "y": 1,
            "stack-level": 0,
            "predicates": ["iscuttable"],
            "id": "a"
        }
    ],
    "players": [
        {
            "name": "robot",
            "x": 0,
            "y": 0,
            "direction": [0, 1]
        }
    ],
    "goal_description": "Cut the lettuce on the board until it is cut",
    "goal": [
        {
            "predicate": "iscut",
            "args": ["lettuce"],
            "ids": ["a"]
        }
    ]
}
        \end{minted}
        \end{tcolorbox}

        \vspace{1em}  % Space between stacked JSONs

        % Second stacked JSON
        \begin{tcolorbox}[colframe=black, boxrule=0.5mm, width=\textwidth, boxsep=0pt, left=0pt, right=0pt, top=0pt, bottom=0pt]
        \begin{minted}[fontsize=\scriptsize, breaklines, frame=none, bgcolor=white,
            xleftmargin=0pt, xrightmargin=0pt, texcomments=true, escapeinside=||,
            highlightlines=true, style=colorful, 
            highlightcolor=\color{red}, highlightcolor=\color{green}] {json}
{
    "mouse_click_actions": [
        {
            "name": "move",
            "input_instructions": {
                "button": "left",
                "click_on": "s2"
            }
        },...
    ],
    "keyboard_actions": [
        {
            "name": "cook",
            "input_instructions": {
                "key": "e",
                "at": "s1"
            }
        },...
    ]
}
        \end{minted}
        \end{tcolorbox}
    \end{minipage}
    
    \caption{Combined JSONs: (Left) Rendering JSON, (Top-right) Environment JSON, (Bottom-right) Input JSON.}
    \label{fig:combined_jsons}
\end{figure}
